# Supplementary material for: Optimal Mixture Weights for Off-Policy Evaluation with Multiple Behavior Policies
Source: arXiv:2011.14359 source file (2020-11-29)
Supplement: Supplementary file 1 [file appendix.pdf]

## 308 **A Proof of Theorems and Propositions**

### 309 **A.1 Proof of Theorem 1**

310 The variance of a mixture estimator is

$$\mathbb{V}[\hat{V}_\alpha] = \sum_{i=1}^M \alpha_i^2 \mathbb{V}[\hat{V}_i].$$

311 The variance of  $\hat{V}_{MIX}$  is

$$\begin{aligned} \mathbb{V}[\hat{V}_{MIX}] &= \sum_{i=1}^M \frac{1}{(\mathbb{V}[\hat{V}_i] \sum_{j=1}^M \frac{1}{\mathbb{V}[\hat{V}_j]})^2} \mathbb{V}[\hat{V}_i] \\ &= \frac{1}{\sum_{i=1}^M \frac{1}{\mathbb{V}[\hat{V}_i]}}. \end{aligned} \quad (11)$$

312 Therefore,

$$\begin{aligned} \frac{\mathbb{V}[\hat{V}_\alpha]}{\mathbb{V}[\hat{V}_{MIX}]} &= \sum_{i=1}^M \frac{1}{\mathbb{V}[\hat{V}_i]} \sum_{i=1}^M \alpha_i^2 \mathbb{V}[\hat{V}_i] \\ &\geq \left( \sum_{i=1}^M |\alpha_i| \right)^2 \\ &\geq \left( \sum_{i=1}^M \alpha_i \right)^2 = 1. \end{aligned} \quad (12)$$

313 This means that any mixture estimator other than  $\hat{V}_{MIX}$  has higher or equal variance.

### 314 **A.2 Proof of Proposition 1**

315 The unbiasedness is proved as

$$\begin{aligned} \mathbb{E}[\hat{V}_{MIXT} - V] &= \mathbb{E}\left[\sum_{t=0}^T \sum_{i=1}^M \alpha_{i,t} \hat{V}_{i,t} - \sum_{t=0}^T V_t\right] \\ &= \mathbb{E}\left[\sum_{t=0}^T \sum_{i=1}^M \alpha_{i,t} (\hat{V}_{i,t} - V_t)\right] \\ &= \sum_{t=0}^T \sum_{i=1}^M \alpha_{i,t} \mathbb{E}[(\hat{V}_{i,t} - V_t)] \\ &= 0. \end{aligned} \quad (13)$$

316 The variance of  $\hat{V}_{MIXT}$  is

$$\mathbb{V}[\hat{V}_{MIXT}] = \sum_{i=1}^M \left( \sum_{t=0}^T \alpha_{i,t}^2 \mathbb{V}[\hat{V}_{i,t}] + 2 \sum_{1 \leq t_1 < t_2 \leq T} \alpha_{i,t_1} \alpha_{i,t_2} \text{Cov}[\hat{V}_{i,t_1}, \hat{V}_{i,t_2}] \right), \quad (14)$$

317 where  $\forall t, \sum_{i=1}^M \alpha_{i,t} = 1$ . We construct the Lagrangian function for the problem

$$\mathcal{L}[A, \Lambda] = \sum_{i=1}^M \left( \sum_{t=0}^T \alpha_{i,t}^2 \mathbb{V}[\hat{V}_{i,t}] + 2 \sum_{1 \leq t_1 < t_2 \leq T} \alpha_{i,t_1} \alpha_{i,t_2} \text{Cov}[\hat{V}_{i,t_1}, \hat{V}_{i,t_2}] \right) - \sum_{t=0}^T \lambda_t \left( \sum_{i=1}^M \alpha_{i,t} - 1 \right), \quad (15)$$

where  $\lambda_t$  are Lagrangian multipliers. Let  $\frac{\partial \mathcal{L}}{\partial \alpha_{i,t}} = 0$  and  $\frac{\partial \mathcal{L}}{\partial \lambda_t} = 0$ , we get

$$\forall i \forall t \quad 2\mathbb{V}[\hat{V}_{i,t}]\alpha_{i,t} + 2 \sum_{\tau \neq t} \alpha_{i,\tau} \text{Cov}[\hat{V}_{i,t}, \hat{V}_{i,\tau}] = \lambda_t, \quad (16)$$

$$\forall t \quad \sum_{i=1}^M \alpha_{i,t} = 1. \quad (17)$$

We denote  $[\lambda_0, \lambda_1, \dots, \lambda_T]^T$  by  $\vec{\lambda}$ . From (16) we know that  $\forall i \quad 2\Sigma_i \vec{\alpha}_i^* = \vec{\lambda}$ , which means  $\forall i \quad \vec{\alpha}_i^* = \frac{1}{2}\Sigma_i^{-1}\vec{\lambda}$ . Add up (17), and we get  $\vec{e} = \sum_{i=1}^M \vec{\alpha}_i^* = \frac{1}{2} \sum_{i=1}^M \Sigma_i^{-1} \vec{\lambda}$ , which means  $\frac{1}{2} \vec{\lambda} = (\sum_{i=1}^M \Sigma_i^{-1})^{-1} \vec{e}$ . Therefore,  $\forall i \quad \vec{\alpha}_i^* = \Sigma_i^{-1} (\sum_{i=1}^M \Sigma_i^{-1})^{-1} \vec{e}$ . We have found a stationary point of (14), so now we need to show that it is the global minima. Note that the solutions of (17) forms a convex set on  $R^{M \times T}$ . In addition, because all the covariance matrixes are positive definite,  $\mathbb{V}[\hat{V}_{MIXT}]$  is also a strictly convex function of  $\vec{\alpha}$ . Therefore,  $\vec{\alpha}_i^*$  are the local minima as well as the global minima.

To prove the variance reduction, we rewrite  $\hat{V}_{MIX}$  as

$$\hat{V}_{MIX} = \sum_{i=1}^M \sum_{t=0}^T \alpha_i V_{i,t}. \quad (18)$$

Note that  $\alpha_{i,t}$  are the optimal mixture weights to minimize variance, so  $\mathbb{V}[\hat{V}_{MIXT}] \leq \mathbb{V}[\hat{V}_{MIX}]$ .

### A.3 Proof of Proposition 2

The variance of  $V_{MIXC}$  is

$$\begin{aligned} \mathbb{V}[\hat{V}_{MIXC}] &= \sum_{i=1}^M \sum_{t_1=0}^T \sum_{t_2=0}^T (\alpha_{i,t_1} \alpha_{i,t_2} \text{Cov}[\hat{V}_{i,t_1}, \hat{V}_{i,t_2}] + \beta_{i,t_1} \beta_{i,t_2} \text{Cov}[\hat{W}_{i,t_1}, \hat{W}_{i,t_2}] \\ &\quad + \alpha_{i,t_1} \beta_{i,t_2} \text{Cov}[\hat{V}_{i,t_1}, \hat{W}_{i,t_2}] + \beta_{i,t_1} \alpha_{i,t_2} \text{Cov}[\hat{W}_{i,t_1}, \hat{V}_{i,t_2}]). \end{aligned} \quad (19)$$

Like in A.2 We construct the Lagrangian function for it by

$$\begin{aligned} \mathcal{L}[A, B, \Lambda] &= \sum_{i=1}^M \sum_{t_1=0}^T \sum_{t_2=0}^T (\alpha_{i,t_1} \alpha_{i,t_2} \text{Cov}[\hat{V}_{i,t_1}, \hat{V}_{i,t_2}] + \beta_{i,t_1} \beta_{i,t_2} \text{Cov}[\hat{W}_{i,t_1}, \hat{W}_{i,t_2}] \\ &\quad + \alpha_{i,t_1} \beta_{i,t_2} \text{Cov}[\hat{V}_{i,t_1}, \hat{W}_{i,t_2}] + \beta_{i,t_1} \alpha_{i,t_2} \text{Cov}[\hat{W}_{i,t_1}, \hat{V}_{i,t_2}]) \\ &\quad - \sum_{t=0}^T \lambda_t (\sum_{i=1}^M \alpha_{i,t} - 1). \end{aligned} \quad (20)$$

Let  $\frac{\partial \mathcal{L}}{\partial \alpha} = 0$ ,  $\frac{\partial \mathcal{L}}{\partial \beta} = 0$ ,  $\frac{\partial \mathcal{L}}{\partial \Lambda} = 0$ , we have

$$\forall i, \quad 2 \begin{pmatrix} \vec{\alpha}_i^* \\ \vec{\beta}_i^* \end{pmatrix} = \begin{pmatrix} H_{i,11} & H_{i,12} \\ H_{i,21} & H_{i,22} \end{pmatrix} \begin{pmatrix} \vec{\lambda} \\ \vec{0} \end{pmatrix}, \quad (21)$$

$$\forall t \quad \sum_{i=1}^M \alpha_{i,t} = 1. \quad (22)$$

By (22) we can get  $\vec{e} = \sum_{i=1}^M \vec{\alpha}_i^* = \frac{1}{2} \sum_{i=1}^M H_{i,11} \vec{\lambda}$  and compute  $\vec{\lambda}$ . Bringing it to (21), we get  $\vec{\alpha}_i^* = H_{i,11} (\sum_{j=1}^M H_{j,11})^{-1} \vec{e}$  and  $\vec{\beta}_i^* = H_{i,21} (\sum_{j=1}^M H_{j,11})^{-1} \vec{e}$ . Similar to A.2, we can prove that this stationary point is the global minima.

## B Delta Method

### B.1 Derivation of Delta Method

In this section, we introduce Delta Method [18], which is used for estimating the variance of WIS and WDR. Given a function of expectations of random variables  $\theta = f(\mathbb{E}[\mathbf{X}])$ , it is usually hard to obtain

an unbiased estimator. Luckily, if  $f$  is a continuous function, the empirical estimation  $\hat{\theta} = f(\bar{\mathbf{X}})$ , where  $\bar{\mathbf{X}}$  is the sample mean of data, is strongly consistent. However, the samples are inside the function so the variance of  $\hat{\theta}$  is hard to determine. We present the technology in Owen [18] here to build the framework of estimating variance for  $\hat{\theta}$ .

By first order Taylor expansion of  $f$ ,  $\hat{\theta}$  is approximated by

$$\hat{\theta} \approx \theta + \sum_{i=1}^d (\bar{X}_i - \mu_i) f_i(\mu), \quad (23)$$

where  $X_i$  is the  $i$ -th component of  $\mathbf{X}$ ,  $\mu_i = \mathbb{E}[X_i]$ , and  $f_i = \frac{\partial f}{\partial X_i}$ . When the sample size  $n$  is large,  $\bar{X}_i$  is very close to  $\mu_i$ , so the right hand side is a good approximate of  $\hat{\theta}$ . The variance of  $\hat{\theta}$  is then approximated by

$$\mathbb{V}[\hat{\theta}] \approx \frac{1}{n} \left( \sum_{i=1}^d f_i(\mu)^2 \sigma_i^2 + 2 \sum_{i=1}^{d-1} \sum_{j=i+1}^d f_i(\mu) f_j(\mu) \sigma_{i,j} \right) = \frac{1}{n} (\nabla f)^T \Sigma (\nabla f), \quad (24)$$

where  $\sigma_i^2$  is the variance of  $X_i$ ,  $\sigma_{i,j}$  is the covariance of  $X_i$  and  $X_j$ ,  $\nabla f$  is the gradient of  $f$  and  $\Sigma$  is the corresponding covariance matrix.

## B.2 Variance of Weighted Estimators

We estimate the variance of weighted estimators by (24). Define  $\theta = f(\mu_x, \mu_y) = \frac{\mu_y}{\mu_x}$ , where  $\mu_x = \mathbb{E}[\mathbf{X}]$  and  $\mu_y = \mathbb{E}[\mathbf{Y}]$ , then  $f_x = -\frac{\mu_y}{\mu_x^2}$ ,  $f_y = \frac{1}{\mu_x}$ . If we define  $\sigma_x^2 = \mathbb{V}[\mathbf{X}]$ ,  $\sigma_y^2 = \mathbb{V}[\mathbf{Y}]$ , and  $\sigma_{x,y} = \text{Cov}[\mathbf{X}, \mathbf{Y}]$ ,  $\mathbb{V}[\hat{\theta}]$  is approximated by

$$\begin{aligned} \mathbb{V}[\hat{\theta}] &= \frac{1}{n} \left( \frac{\mu_y^2 \sigma_x^2}{\mu_x^4} + \frac{\sigma_y^2}{\mu_x^2} - \frac{2\mu_y \sigma_{x,y}}{\mu_x^3} \right) \\ &= \frac{1}{n} \frac{\theta^2 \sigma_x^2 + \sigma_y^2 - 2\theta \sigma_{x,y}}{\mu_x^2} \\ &= \frac{1}{n} \frac{\theta^2 \sigma_x^2 + \sigma_y^2 - 2\theta \sigma_{x,y} + (\mu_y - \theta \mu_x)^2}{\mu_x^2} \\ &= \frac{1}{n} \frac{\mathbb{E}[\theta^2 \mathbf{X}^2] + \mathbb{E}[\mathbf{Y}^2] - 2\mathbb{E}[\theta \mathbf{X} \mathbf{Y}]}{\mu_x^2} \\ &= \frac{1}{n} \frac{\mathbb{E}[(\theta \mathbf{X} - \mathbf{Y})^2]}{\mu_x^2}. \end{aligned} \quad (25)$$

## B.3 Covariance of Weighted Estimators

To estimate the covariance, we define  $\theta_1 = f(\mu_{x_1}, \mu_{y_1}) = \frac{\mu_{y_1}}{\mu_{x_1}}$  and  $\theta_2 = f(\mu_{x_2}, \mu_{y_2}) = \frac{\mu_{y_2}}{\mu_{x_2}}$ . The corresponding expectations, variances and covariances are represented by  $\mu_{x_1}, \mu_{y_1}, \mu_{x_2}, \mu_{y_2}, \sigma_{x_1}^2, \sigma_{y_1}^2, \sigma_{x_2}^2, \sigma_{y_2}^2, \sigma_{x_1, x_2}, \sigma_{x_1, y_2}, \sigma_{y_1, x_2}, \sigma_{y_1, y_2}$ . The covariance approximation  $\text{Cov}[\hat{\theta}_1, \hat{\theta}_2]$  is

$$\begin{aligned} \text{Cov}[\hat{\theta}_1, \hat{\theta}_2] &= \frac{1}{n} \left( \frac{\mu_{y_1} \mu_{y_2} \sigma_{x_1, x_2}}{\mu_{x_1}^2 \mu_{x_2}^2} - \frac{\mu_{y_1} \sigma_{x_1, y_2}}{\mu_{x_1}^2 \mu_{x_2}} - \frac{\mu_{y_2} \sigma_{y_1, x_2}}{\mu_{x_1} \mu_{x_2}^2} + \frac{\sigma_{y_1, y_2}}{\mu_{x_1} \mu_{x_2}} \right) \\ &= \frac{1}{n} \frac{\theta_1 \theta_2 \sigma_{x_1, x_2} - \theta_1 \sigma_{x_1, y_2} - \theta_2 \sigma_{y_1, x_2} + \sigma_{y_1, y_2}}{\mu_{x_1} \mu_{x_2}} \\ &= \frac{1}{n} \frac{\theta_1 \theta_2 \sigma_{x_1, x_2} - \theta_1 \sigma_{x_1, y_2} - \theta_2 \sigma_{y_1, x_2} + \sigma_{y_1, y_2} + (\mu_{y_1} - \theta_1 \mu_{x_1})(\mu_{y_2} - \theta_2 \mu_{x_2})}{\mu_{x_1} \mu_{x_2}} \\ &= \frac{1}{n} \frac{\mathbb{E}[\theta_1 \theta_2 \mathbf{X}_1 \mathbf{X}_2] - \mathbb{E}[\theta_1 \mathbf{X}_1 \mathbf{Y}_2] - \mathbb{E}[\theta_2 \mathbf{Y}_1 \mathbf{X}_2] + \mathbb{E}[\mathbf{Y}_1 \mathbf{Y}_2]}{\mu_{x_1} \mu_{x_2}} \\ &= \frac{1}{n} \frac{\mathbb{E}[(\theta_1 \mathbf{X}_1 - \mathbf{Y}_1)(\theta_2 \mathbf{X}_2 - \mathbf{Y}_2)]}{\mu_{x_1} \mu_{x_2}}. \end{aligned} \quad (26)$$

### 357 B.4 Variance of Summation of Weighted Estimators

358 We use the formulas in [B.2](#) and [B.3](#) to derive the variance of summation of weighted estimators.  
 359 Define  $\theta = g(\mu_{x_1}, \mu_{y_1}, \mu_{x_2}, \mu_{y_2}, \dots, \mu_{x_T}, \mu_{y_T}) = \sum_{t=0}^T \theta_t = \sum_{t=0}^T \frac{\mu_{y_t}}{\mu_{x_t}}$ , where  $\mu_{x_t} = \mathbb{E}[\mathbf{X}_t]$  and  
 360  $\mu_{y_t} = \mathbb{E}[\mathbf{Y}_t]$ . Then

$$\begin{aligned} \mathbb{V}[\hat{\theta}] &\approx \sum_{t=0}^T \mathbb{V}[\hat{\theta}_t] + 2 \sum_{t=0}^{T-1} \sum_{\tau=t+1}^T \text{Cov}[\hat{\theta}_t, \hat{\theta}_\tau] \\ &= \frac{1}{n} \left( \sum_{t=0}^T \frac{\mathbb{E}[(\theta_t \mathbf{X}_t - \mathbf{Y}_t)^2]}{\mu_{x_t}^2} + 2 \sum_{t=0}^{T-1} \sum_{\tau=t+1}^T \frac{\mathbb{E}[(\theta_t \mathbf{X}_t - \mathbf{Y}_t)(\theta_\tau \mathbf{Y}_\tau - \mathbf{X}_\tau)]}{\mu_{x_t} \mu_{x_\tau}} \right) \\ &= \frac{1}{n} \mathbb{E} \left[ \left( \sum_{t=0}^T \frac{\theta_t \mathbf{X}_t - \mathbf{Y}_t}{\mu_{x_t}} \right)^2 \right]. \end{aligned} \quad (27)$$

361 If we add the subscript  $i$  to the formula, the formula would be

$$\mathbb{V}[\hat{V}_i] \approx \frac{1}{n_i} \mathbb{E} \left[ \left( \sum_{t=0}^T \frac{\theta_{i,t} \mathbf{X}_{i,t} - \mathbf{Y}_{i,t}}{\mu_{x_{i,t}}} \right)^2 \right]. \quad (28)$$

362 If we use the samples  $X_{i,j,t}$  and  $Y_{i,j,t}$  to estimate  $\mathbb{V}[\hat{V}_i]$ , the estimated variance would be

$$\begin{aligned} \text{Var}_i &= \frac{1}{n_i^2} \sum_{j=1}^{n_i} \left( \sum_{t=0}^T \frac{\hat{Y}_{i,j,t} - \hat{\theta}_{i,t} \hat{X}_{i,j,t}}{\frac{1}{n_i} \sum_{k=1}^{n_i} \hat{X}_{i,k,t}} \right)^2 \\ &= \sum_{j=1}^{n_i} \left( \sum_{t=0}^T \frac{\hat{Y}_{i,j,t} - \hat{\theta}_{i,t} \hat{X}_{i,j,t}}{\sum_{k=1}^{n_i} \hat{X}_{i,k,t}} \right)^2. \end{aligned} \quad (29)$$

363 We now show that  $n_i * \text{Var}_i$  is strongly consistent. It is derived as

$$\begin{aligned} n_i * \text{Var}_i &= \frac{1}{n_i} \sum_{j=1}^{n_i} \left( \sum_{t=0}^T \frac{\hat{Y}_{i,j,t} - \hat{\theta}_{i,t} \hat{X}_{i,j,t}}{\frac{1}{n_i} \sum_{k=1}^{n_i} \hat{X}_{i,k,t}} \right)^2 \\ &= \frac{1}{n_i} \sum_{j=1}^{n_i} \sum_{t=0}^T \sum_{\tau=0}^T \frac{\hat{Y}_{i,j,t} - \hat{\theta}_{i,t} \hat{X}_{i,j,t}}{\frac{1}{n_i} \sum_{k=1}^{n_i} \hat{X}_{i,k,t}} \cdot \frac{\hat{Y}_{i,j,\tau} - \hat{\theta}_{i,\tau} \hat{X}_{i,j,\tau}}{\frac{1}{n_i} \sum_{k=1}^{n_i} \hat{X}_{i,k,\tau}} \\ &= \sum_{t=0}^T \sum_{\tau=0}^T \frac{\frac{1}{n_i} \sum_{j=1}^{n_i} (\hat{Y}_{i,j,t} - \hat{\theta}_{i,t} \hat{X}_{i,j,t})(\hat{Y}_{i,j,\tau} - \hat{\theta}_{i,\tau} \hat{X}_{i,j,\tau})}{\frac{1}{n_i} \sum_{k=1}^{n_i} \hat{X}_{i,k,t} \cdot \frac{1}{n_i} \sum_{k=1}^{n_i} \hat{X}_{i,k,\tau}} \\ &= \sum_{t=0}^T \sum_{\tau=0}^T \frac{\frac{1}{n_i} \sum_{j=1}^{n_i} \hat{Y}_{i,j,t} \hat{Y}_{i,j,\tau} + \frac{\hat{\theta}_{i,t} \hat{\theta}_{i,\tau}}{n_i} \sum_{j=1}^{n_i} \hat{X}_{i,j,t} \hat{X}_{i,j,\tau}}{\frac{1}{n_i} \sum_{k=1}^{n_i} \hat{X}_{i,k,t} \cdot \frac{1}{n_i} \sum_{k=1}^{n_i} \hat{X}_{i,k,\tau}} \\ &\quad - \frac{\frac{\hat{\theta}_{i,t}}{n_i} \sum_{j=1}^{n_i} \hat{X}_{i,j,t} \hat{Y}_{i,j,\tau} + \frac{\hat{\theta}_{i,\tau}}{n_i} \sum_{j=1}^{n_i} \hat{X}_{i,j,\tau} \hat{Y}_{i,j,t}}{\frac{1}{n_i} \sum_{k=1}^{n_i} \hat{X}_{i,k,t} \cdot \frac{1}{n_i} \sum_{k=1}^{n_i} \hat{X}_{i,k,\tau}}. \end{aligned} \quad (30)$$

364 Therefore,  $n_i * \text{Var}_i$  is strongly consistent for

$$\begin{aligned} E_i &= \sum_{t=0}^T \sum_{\tau=0}^T \frac{\mathbb{E}[\mathbf{Y}_{i,t} \mathbf{Y}_{i,\tau}] + \theta_{i,t} \theta_{i,\tau} \mathbb{E}[\mathbf{X}_{i,t} \mathbf{X}_{i,\tau}] - \theta_{i,t} \mathbb{E}[\mathbf{X}_{i,t} \mathbf{Y}_{i,\tau}] - \theta_{i,\tau} \mathbb{E}[\mathbf{X}_{i,\tau} \mathbf{Y}_{i,t}]}{\mu_{x_{i,t}} \mu_{x_{i,\tau}}} \\ &= \sum_{t=0}^T \sum_{\tau=0}^T \frac{\mathbb{E}[(\mathbf{Y}_{i,t} - \theta_{i,t} \mathbf{X}_{i,t})(\mathbf{Y}_{i,\tau} - \theta_{i,\tau} \mathbf{X}_{i,\tau})]}{\mu_{x_{i,t}} \mu_{x_{i,\tau}}} \\ &= \mathbb{E} \left[ \left( \sum_{t=0}^T \frac{\mathbf{Y}_{i,t} - \theta_{i,t} \mathbf{X}_{i,t}}{\mu_{x_{i,t}}} \right)^2 \right]. \end{aligned} \quad (31)$$

## 365 B.5 Covariance of Summation of two Weighted Estimators

366 Similarly, we can estimate the covariance of  $\hat{\theta}_1$  and  $\hat{\theta}_2$ , where  $\hat{\theta}_1$  estimates  $\theta_1 =$   
 367  $g(\mu_{w_1}, \mu_{x_1}, \mu_{y_1}, \mu_{z_1}) = \frac{\mu_{x_1}}{\mu_{w_1}} + \frac{\mu_{z_1}}{\mu_{y_1}}$  and  $\hat{\theta}_2$  estimates  $\theta_2 = g(\mu_{w_2}, \mu_{x_2}, \mu_{y_2}, \mu_{z_2}) = \frac{\mu_{x_2}}{\mu_{w_2}} + \frac{\mu_{z_2}}{\mu_{y_2}}$ .  
 368 Define  $\theta_{11} = \frac{\mu_{x_1}}{\mu_{w_1}}$ ,  $\theta_{12} = \frac{\mu_{z_1}}{\mu_{y_1}}$ ,  $\theta_{21} = \frac{\mu_{x_2}}{\mu_{w_2}}$ ,  $\theta_{22} = \frac{\mu_{z_2}}{\mu_{y_2}}$ , then

$$\begin{aligned} Cov[\hat{\theta}_1, \hat{\theta}_2] &= Cov[\hat{\theta}_{11}, \hat{\theta}_{21}] + Cov[\hat{\theta}_{11}, \hat{\theta}_{22}] + Cov[\hat{\theta}_{12}, \hat{\theta}_{21}] + Cov[\hat{\theta}_{12}, \hat{\theta}_{22}] \\ &= \frac{1}{n} \left( \frac{\mathbb{E}[(\theta_{11}\mathbf{W}_1 - \mathbf{X}_1)(\theta_{21}\mathbf{W}_2 - \mathbf{X}_2)]}{\mu_{w_1}\mu_{w_2}} + \frac{\mathbb{E}[(\theta_{11}\mathbf{W}_1 - \mathbf{X}_1)(\theta_{22}\mathbf{Y}_2 - \mathbf{Z}_2)]}{\mu_{w_1}\mu_{y_2}} + \right. \\ &\quad \left. \frac{\mathbb{E}[(\theta_{12}\mathbf{Y}_1 - \mathbf{Z}_1)(\theta_{21}\mathbf{W}_2 - \mathbf{X}_2)]}{\mu_{y_1}\mu_{w_2}} + \frac{\mathbb{E}[(\theta_{12}\mathbf{Y}_1 - \mathbf{Z}_1)(\theta_{22}\mathbf{Y}_2 - \mathbf{Z}_2)]}{\mu_{y_1}\mu_{y_2}} \right) \\ &= \frac{1}{n} \mathbb{E} \left[ \left( \frac{\theta_{11}\mathbf{W}_1 - \mathbf{X}_1}{\mu_{w_1}} + \frac{\theta_{12}\mathbf{Y}_1 - \mathbf{Z}_1}{\mu_{y_1}} \right) \left( \frac{\theta_{21}\mathbf{W}_2 - \mathbf{X}_2}{\mu_{w_2}} + \frac{\theta_{22}\mathbf{Y}_2 - \mathbf{Z}_2}{\mu_{y_2}} \right) \right]. \quad (32) \end{aligned}$$

369 If we add the subscript  $i$ , replace the subscript of 1 by  $t_1$  and 2 by  $t_2$ , and let  $\theta_{11} = \nu_{i,t_1}$ ,  $\theta_{12} = \omega_{i,t_1}$ ,  
 370  $\theta_{21} = \nu_{i,t_2}$ ,  $\theta_{22} = \omega_{i,t_2}$ , then

$$\begin{aligned} Cov[\hat{V}_{i,t_1}, \hat{V}_{i,t_2}] &= \frac{1}{n_i} \mathbb{E} \left[ \left( \frac{\nu_{i,t_1}\mathbf{W}_{i,t_1} - \mathbf{X}_{i,t_1}}{\mu_{w_{i,t_1}}} + \frac{\omega_{i,t_1}\mathbf{Y}_{i,t_1} - \mathbf{Z}_{i,t_1}}{\mu_{y_{i,t_1}}} \right) \left( \frac{\nu_{i,t_2}\mathbf{W}_{i,t_2} - \mathbf{X}_{i,t_2}}{\mu_{w_{i,t_2}}} + \frac{\omega_{i,t_2}\mathbf{Y}_{i,t_2} - \mathbf{Z}_{i,t_2}}{\mu_{y_{i,t_2}}} \right) \right]. \quad (33) \end{aligned}$$

371 If we use samples to estimate the covariance, the estimator will be

$$\begin{aligned} Cov_{i,t_1,t_2} &= \sum_{j=1}^{n_i} \left( \frac{\hat{X}_{i,j,t_1} - \hat{\nu}_{i,t_1}\hat{W}_{i,j,t_1}}{\sum_{k=1}^{n_i} \hat{W}_{i,k,t_1}} + \frac{\hat{Z}_{i,j,t_1} - \hat{\omega}_{i,t_1}\hat{Y}_{i,j,t_1}}{\sum_{k=1}^{n_i} \hat{Y}_{i,k,t_1}} \right) \\ &\quad \left( \frac{\hat{X}_{i,j,t_2} - \hat{\nu}_{i,t_2}\hat{W}_{i,j,t_2}}{\sum_{k=1}^{n_i} \hat{W}_{i,k,t_2}} + \frac{\hat{Z}_{i,j,t_2} - \hat{\omega}_{i,t_2}\hat{Y}_{i,j,t_2}}{\sum_{k=1}^{n_i} \hat{Y}_{i,k,t_2}} \right). \quad (34) \end{aligned}$$

372 Using the same technique as [B.4](#), we can prove that  $n_i * Cov_{i,t_1,t_2}$  is strongly consistent for  $E_{i,t_1,t_2} =$   
 373  $\mathbb{E} \left[ \left( \frac{\nu_{i,t_1}\mathbf{W}_{i,t_1} - \mathbf{X}_{i,t_1}}{\mu_{w_{i,t_1}}} + \frac{\omega_{i,t_1}\mathbf{Y}_{i,t_1} - \mathbf{Z}_{i,t_1}}{\mu_{y_{i,t_1}}} \right) \left( \frac{\nu_{i,t_2}\mathbf{W}_{i,t_2} - \mathbf{X}_{i,t_2}}{\mu_{w_{i,t_2}}} + \frac{\omega_{i,t_2}\mathbf{Y}_{i,t_2} - \mathbf{Z}_{i,t_2}}{\mu_{y_{i,t_2}}} \right) \right].$

## 374 C Formulations for the Estimators

### 375 C.1 General Formulations for the Estimators

376 The naive mixture estimators for the four methods are

$$\hat{V}_{NMIS} = \sum_{i=1}^M \alpha_i \hat{V}_{IS,i} \quad (35)$$

$$\hat{V}_{NMDR} = \sum_{i=1}^M \alpha_i \hat{V}_{DR,i} \quad (36)$$

$$\hat{V}_{NMWIS} = \sum_{i=1}^M \alpha_i \hat{V}_{SWIS,i} \quad (37)$$

$$\hat{V}_{NMWDR} = \sum_{i=1}^M \alpha_i \hat{V}_{SWDR,i} \quad (38)$$

377 After taking  $t$  into account, the mixture estimators for the four methods are

$$\hat{V}_{MIS} = \sum_{i=1}^M \sum_{t=0}^T \alpha_{i,t} \hat{V}_{IS,i,t} \quad (39)$$

$$\hat{V}_{MDR} = \sum_{i=1}^M \sum_{t=0}^T \alpha_{i,t} \hat{V}_{DR,i,t} \quad (40)$$

$$\hat{V}_{MWIS} = \sum_{i=1}^M \sum_{t=0}^T \alpha_{i,t} \hat{V}_{SWIS,i,t} \quad (41)$$

$$\hat{V}_{MWDR} = \sum_{i=1}^M \sum_{t=0}^T \alpha_{i,t} \hat{V}_{SWDR,i,t} \quad (42)$$

378 After splitting the control variates from DR and SWDR, the  $\alpha\beta$  mixture estimators are

$$\hat{V}_{MDR} = \sum_{i=1}^M \sum_{t=0}^T (\alpha_{i,t} \hat{V}_{IS,i,t} + \beta_{i,t} \hat{W}_{DR,i,t}) \quad (43)$$

$$\hat{V}_{MWDR} = \sum_{i=1}^M \sum_{t=0}^T (\alpha_{i,t} \hat{V}_{SWIS,i,t} + \beta_{i,t} \hat{W}_{SWDR,i,t}) \quad (44)$$

## 379 C.2 Components of the Estimators

380 The sub-estimators in Appendix C.1 are listed below:

| Method | Target               | Formulation                                                                                                                                                        |
|--------|----------------------|--------------------------------------------------------------------------------------------------------------------------------------------------------------------|
| IS     | $\hat{V}_{IS,i}$     | $\frac{1}{n_i} \sum_{j=1}^{n_i} \sum_{t=0}^T \gamma^t \rho_{i,j,t} r_{i,j,t}$                                                                                      |
| IS     | $\hat{V}_{IS,i,t}$   | $\frac{1}{n_i} \sum_{j=1}^{n_i} \gamma^t \rho_{i,j,t} r_{i,j,t}$                                                                                                   |
| DR     | $\hat{V}_{DR,i}$     | $\frac{1}{n_i} \sum_{j=1}^{n_i} \sum_{t=0}^T \gamma^t \left( \rho_{i,j,t-1} \hat{V}(s_{i,j,t}) + \rho_{i,j,t} (r_{i,j,t} - \hat{Q}(s_{i,j,t}, a_{i,j,t})) \right)$ |
| DR     | $\hat{V}_{DR,i,t}$   | $\frac{1}{n_i} \sum_{j=1}^{n_i} \gamma^t \left( \rho_{i,j,t-1} \hat{V}(s_{i,j,t}) + \rho_{i,j,t} (r_{i,j,t} - \hat{Q}(s_{i,j,t}, a_{i,j,t})) \right)$              |
| DR     | $\hat{W}_{DR,i,t}$   | $\frac{1}{n_i} \sum_{j=1}^{n_i} \gamma^t \left( \rho_{i,j,t-1} \hat{V}(s_{i,j,t}) - \rho_{i,j,t} \hat{Q}(s_{i,j,t}, a_{i,j,t}) \right)$                            |
| SWIS   | $\hat{V}_{SWIS,i}$   | $\sum_{j=1}^{n_i} \sum_{t=0}^T \gamma^t u_{i,j,t} r_{i,j,t}$                                                                                                       |
| SWIS   | $\hat{V}_{SWIS,i,t}$ | $\sum_{j=1}^{n_i} \gamma^t u_{i,j,t} r_{i,j,t}$                                                                                                                    |
| SWDR   | $\hat{V}_{SWDR,i}$   | $\sum_{j=1}^{n_i} \sum_{t=0}^T \gamma^t \left( u_{i,j,t-1} \hat{V}(s_{i,j,t}) + u_{i,j,t} (r_{i,j,t} - \hat{Q}(s_{i,j,t}, a_{i,j,t})) \right)$                     |
| SWDR   | $\hat{V}_{SWDR,i,t}$ | $\sum_{j=1}^{n_i} \gamma^t \left( u_{i,j,t-1} \hat{V}(s_{i,j,t}) + u_{i,j,t} (r_{i,j,t} - \hat{Q}(s_{i,j,t}, a_{i,j,t})) \right)$                                  |
| SWDR   | $\hat{W}_{SWDR,i,t}$ | $\sum_{j=1}^{n_i} \gamma^t \left( u_{i,j,t-1} \hat{V}(s_{i,j,t}) - u_{i,j,t} \hat{Q}(s_{i,j,t}, a_{i,j,t}) \right)$                                                |

Table 2: Formulas for the components of the estimators.

## 381 C.3 Variance / Covariance Estimators for the Components

382 We can directly estimate the variances / covariances of components of IS and DR. In addition, with  
 383 the formulas in Appendix B.4 and B.5, we can obtain the variance / covariance estimators for the  
 384 components of SWIS and SWDR.

385 For naive mixture estimators, we need to estimate  $\mathbb{V}[\hat{V}_{IS,i}]$ ,  $\mathbb{V}[\hat{V}_{DR,i}]$ ,  $\mathbb{V}[\hat{V}_{SWIS,i}]$  and  $\mathbb{V}[\hat{V}_{SWDR,i}]$ .  
 386 They are formulated as

$$n_i \mathbb{V}[\hat{V}_{IS,i}] \approx \frac{1}{n_i} \sum_{j=1}^{n_i} \left( \sum_{t=0}^T \gamma^t \rho_{i,j,t} r_{i,j,t} \right)^2 - \left( \frac{1}{n_i} \sum_{j=1}^{n_i} \sum_{t=0}^T \gamma^t \rho_{i,j,t} r_{i,j,t} \right)^2 \quad (45)$$

$$n_i \mathbb{V}[\hat{V}_{DR,i}] \approx \frac{1}{n_i} \sum_{j=1}^{n_i} \left( \sum_{t=0}^T \gamma^t \left( \rho_{i,j,t-1} \hat{V}(s_{i,j,t}) + \rho_{i,j,t} (r_{i,j,t} - \hat{Q}(s_{i,j,t}, a_{i,j,t})) \right) \right)^2 \\ - \left( \frac{1}{n_i} \sum_{j=1}^{n_i} \sum_{t=0}^T \gamma^t \left( \rho_{i,j,t-1} \hat{V}(s_{i,j,t}) + \rho_{i,j,t} (r_{i,j,t} - \hat{Q}(s_{i,j,t}, a_{i,j,t})) \right) \right)^2 \quad (46)$$

$$n_i \mathbb{V}[\hat{V}_{SWIS,i}] \approx n_i \sum_{j=1}^{n_i} \left( \sum_{t=0}^T u_{i,j,t} \left( \gamma^t r_{i,j,t} - \hat{\theta}_{i,t} \right) \right)^2 \quad (47)$$

$$n_i \mathbb{V}[\hat{V}_{SWDR,i}] \approx n_i \sum_{j=1}^{n_i} \left( \sum_{t=0}^T u_{i,j,t} \left( \gamma^t (r_{i,j,t} - \hat{Q}(s_{i,j,t}, a_{i,j,t})) - \hat{\nu}_{i,t} \right) \right. \\ \left. + \sum_{t=0}^T u_{i,j,t-1} \left( \gamma^t \hat{V}(s_{i,j,t}) - \hat{\omega}_{i,t} \right) \right)^2 \quad (48)$$

387 where  $\hat{\theta}_{i,t} = \sum_{j=1}^{n_i} \gamma^t u_{i,j,t} r_{i,j,t}$ ,  $\hat{\nu}_{i,t} = \sum_{j=1}^{n_i} \gamma^t u_{i,j,t} (r_{i,j,t} - \hat{Q}(s_{i,j,t}, a_{i,j,t}))$  and  $\hat{\omega}_{i,t} =$   
 388  $\sum_{j=1}^{n_i} \gamma^t u_{i,j,t-1} \hat{V}(s_{i,j,t})$ .

389 For mixture estimators, we will need to estimate  $Cov[\hat{V}_{IS,i,t_1}, \hat{V}_{IS,i,t_2}]$ ,  $Cov[\hat{V}_{DR,i,t_1}, \hat{V}_{DR,i,t_2}]$ ,  
 390  $Cov[\hat{V}_{SWIS,i,t_1}, \hat{V}_{SWIS,i,t_2}]$  and  $Cov[\hat{V}_{SWDR,i,t_1}, \hat{V}_{SWDR,i,t_2}]$ . Their formulations are

$$n_i Cov[\hat{V}_{IS,i,t_1}, \hat{V}_{IS,i,t_2}] \approx \frac{1}{n_i} \sum_{j=1}^{n_i} \gamma^{t_1+t_2} \rho_{i,j,t_1} \rho_{i,j,t_2} r_{i,j,t_1} r_{i,j,t_2} \\ - \left( \frac{1}{n_i} \sum_{j=1}^{n_i} \gamma^{t_1} \rho_{i,j,t_1} r_{i,j,t_1} \right) \left( \frac{1}{n_i} \sum_{j=1}^{n_i} \gamma^{t_2} \rho_{i,j,t_2} r_{i,j,t_2} \right) \quad (49)$$

$$n_i Cov[\hat{V}_{DR,i,t_1}, \hat{V}_{DR,i,t_2}] \approx \frac{1}{n_i} \sum_{j=1}^{n_i} \left( \gamma^{t_1} \left( \rho_{i,j,t_1-1} \hat{V}(s_{i,j,t_1}) + \rho_{i,j,t_1} (r_{i,j,t_1} - \hat{Q}(s_{i,j,t_1}, a_{i,j,t_1})) \right) \right) \\ * \left( \gamma^{t_2} \left( \rho_{i,j,t_2-1} \hat{V}(s_{i,j,t_2}) + \rho_{i,j,t_2} (r_{i,j,t_2} - \hat{Q}(s_{i,j,t_2}, a_{i,j,t_2})) \right) \right) \\ - \left( \frac{1}{n_i} \sum_{j=1}^{n_i} \gamma^{t_1} \left( \rho_{i,j,t_1-1} \hat{V}(s_{i,j,t_1}) + \rho_{i,j,t_1} (r_{i,j,t_1} - \hat{Q}(s_{i,j,t_1}, a_{i,j,t_1})) \right) \right) \\ * \left( \frac{1}{n_i} \sum_{j=1}^{n_i} \gamma^{t_2} \left( \rho_{i,j,t_2-1} \hat{V}(s_{i,j,t_2}) + \rho_{i,j,t_2} (r_{i,j,t_2} - \hat{Q}(s_{i,j,t_2}, a_{i,j,t_2})) \right) \right) \quad (50)$$

$$n_i Cov[\hat{V}_{SWIS,i,t_1}, \hat{V}_{SWIS,i,t_2}] \approx n_i \sum_{j=1}^{n_i} u_{i,j,t_1} u_{i,j,t_2} \left( \gamma^{t_1} r_{i,j,t_1} - \hat{\theta}_{i,t_1} \right) \left( \gamma^{t_2} r_{i,j,t_2} - \hat{\theta}_{i,t_2} \right) \quad (51)$$

$$\begin{aligned}
n_i \text{Cov}[\hat{V}_{SWDR,i,t_1}, \hat{V}_{SWDR,i,t_2}] &\approx n_i \sum_{j=1}^{n_i} \left( u_{i,j,t_1} \left( \gamma^{t_1} \left( r_{i,j,t_1} - \hat{Q}(s_{i,j,t_1}, a_{i,j,t_1}) \right) - \hat{\nu}_{i,t_1} \right) \right. \\
&\quad \left. + u_{i,j,t_1-1} \left( \gamma^{t_1} \hat{V}(s_{i,j,t_1}) - \hat{\omega}_{i,t_1} \right) \right) \\
&\quad * \left( u_{i,j,t_2} \left( \gamma^{t_2} \left( r_{i,j,t_2} - \hat{Q}(s_{i,j,t_2}, a_{i,j,t_2}) \right) - \hat{\nu}_{i,t_2} \right) \right. \\
&\quad \left. + u_{i,j,t_2-1} \left( \gamma^{t_2} \hat{V}(s_{i,j,t_2}) - \hat{\omega}_{i,t_2} \right) \right) \quad (52)
\end{aligned}$$

392 For  $\alpha\beta$  mixture estimators, we need to estimate  $\text{Cov}[\hat{V}_{IS,i,t_1}, \hat{W}_{DR,i,t_2}]$ ,  $\text{Cov}[\hat{W}_{DR,i,t_1}, \hat{W}_{DR,i,t_2}]$ ,  
 393  $\text{Cov}[\hat{V}_{SWIS,i,t_1}, \hat{W}_{SWDR,i,t_2}]$  and  $\text{Cov}[\hat{W}_{SWDR,i,t_1}, \hat{W}_{SWDR,i,t_2}]$ . They can be approximated by

$$\begin{aligned}
n_i \text{Cov}[\hat{V}_{IS,i,t_1}, \hat{W}_{DR,i,t_2}] &\approx \frac{1}{n_i} \sum_{j=1}^{n_i} \gamma^{t_1+t_2} \rho_{i,j,t_1} r_{i,j,t_1} \left( \rho_{i,j,t_2-1} \hat{V}(s_{i,j,t_2}) - \rho_{i,j,t_2} \hat{Q}(s_{i,j,t_2}, a_{i,j,t_2}) \right) \\
&\quad - \left( \frac{1}{n_i} \sum_{j=1}^{n_i} \gamma^{t_1} \rho_{i,j,t_1} r_{i,j,t_1} \right) \\
&\quad * \left( \frac{1}{n_i} \sum_{j=1}^{n_i} \gamma^{t_2} \left( \rho_{i,j,t_2-1} \hat{V}(s_{i,j,t_2}) - \rho_{i,j,t_2} \hat{Q}(s_{i,j,t_2}, a_{i,j,t_2}) \right) \right) \quad (53)
\end{aligned}$$

$$\begin{aligned}
n_i \text{Cov}[\hat{W}_{DR,i,t_1}, \hat{W}_{DR,i,t_2}] &\approx \frac{1}{n_i} \sum_{j=1}^{n_i} \gamma^{t_1+t_2} \left( \rho_{i,j,t_1-1} \hat{V}(s_{i,j,t_1}) - \rho_{i,j,t_1} \hat{Q}(s_{i,j,t_1}, a_{i,j,t_1}) \right) \\
&\quad * \left( \rho_{i,j,t_2-1} \hat{V}(s_{i,j,t_2}) - \rho_{i,j,t_2} \hat{Q}(s_{i,j,t_2}, a_{i,j,t_2}) \right) \\
&\quad - \left( \frac{1}{n_i} \sum_{j=1}^{n_i} \gamma^{t_1} \left( \rho_{i,j,t_1-1} \hat{V}(s_{i,j,t_1}) - \rho_{i,j,t_1} \hat{Q}(s_{i,j,t_1}, a_{i,j,t_1}) \right) \right) \\
&\quad * \left( \frac{1}{n_i} \sum_{j=1}^{n_i} \gamma^{t_2} \left( \rho_{i,j,t_2-1} \hat{V}(s_{i,j,t_2}) - \rho_{i,j,t_2} \hat{Q}(s_{i,j,t_2}, a_{i,j,t_2}) \right) \right) \quad (54)
\end{aligned}$$

$$\begin{aligned}
n_i \text{Cov}[\hat{V}_{SWIS,i,t_1}, \hat{W}_{SWDR,i,t_2}] &\approx n_i \sum_{j=1}^{n_i} u_{i,j,t_1} \left( \gamma^{t_1} r_{i,j,t_1} - \hat{\theta}_{i,t_1} \right) \\
&\quad * \left( u_{i,j,t_2-1} \left( \gamma^{t_2} \hat{V}(s_{i,j,t_2}) - \hat{\phi}_{i,t_2} \right) - u_{i,j,t_2} \left( \gamma^{t_2} \hat{Q}(s_{i,j,t_2}, a_{i,j,t_2}) - \hat{\psi}_{i,t_2} \right) \right) \quad (55)
\end{aligned}$$

$$\begin{aligned}
n_i \text{Cov}[\hat{W}_{SWDR,i,t_1}, \hat{W}_{SWDR,i,t_2}] &\approx n_i \sum_{j=1}^{n_i} \left( u_{i,j,t_1-1} \left( \gamma^{t_1} \hat{V}(s_{i,j,t_1}) - \hat{\phi}_{i,t_1} \right) - u_{i,j,t_1} \left( \gamma^{t_1} \hat{Q}(s_{i,j,t_1}, a_{i,j,t_1}) - \hat{\psi}_{i,t_1} \right) \right) \\
&\quad * \left( u_{i,j,t_2-1} \left( \gamma^{t_2} \hat{V}(s_{i,j,t_2}) - \hat{\phi}_{i,t_2} \right) - u_{i,j,t_2} \left( \gamma^{t_2} \hat{Q}(s_{i,j,t_2}, a_{i,j,t_2}) - \hat{\psi}_{i,t_2} \right) \right) \quad (56)
\end{aligned}$$

394 where  $\phi_{i,t} = \sum_{j=1}^{n_i} \gamma^t u_{i,j,t} \hat{V}(s_{i,j,t})$  and  $\psi_{i,t} = \sum_{j=1}^{n_i} \gamma^t u_{i,j,t} \hat{Q}(s_{i,j,t}, a_{i,j,t})$ .

395 Note that all of the above estimators multiplied by  $n_i$  are strongly consistent for some value. Therefore,  
 396 we can easily show that the three mixture estimators are all strongly consistent for  $V$ .



## 397 D Experiment Details

### 398 D.1 Environmental Settings

399 In this section, there are no random variables so we use bold letters to denote vectors.

400 In the recommendation environment, we first define the number of topics  $T = 100$ . 1000 documents  
401 are generated and each is observed by a  $T$  dimension vector. Each document should reflect whether it  
402 is related to each topic and each user should indicate the preference of each topic. For the topics, we  
403 generate an abundance vector  $\mathbf{A} = [A_1, A_2, \dots, A_T]^T$  and a quality vector  $\mathbf{Q} = [Q_1, Q_2, \dots, Q_T]^T$ .  
404 The abundance vector satisfies  $\sum_{i=1}^T A_i = 1$  and  $\forall i, A_i \geq 0$ . When we generate a relevant topic  
405 for a document, the abundance vector specifies the probability of generating each topic. The quality  
406 vector satisfies  $\forall i, 0 \leq Q_i \leq 1$ , indicating the original quality of each topic.

407 For each document, we define relevance vector  $\mathbf{r}_i \in \{0, 1\}^T$  and quality  $q_i$ . When the document  
408 sampler is generating the  $i$ -th document, it will first generate three topics  $t_1, t_2$  and  $t_3$  (repeatable) by  
409  $\mathbf{A}$ , and set the  $t_1$ -th,  $t_2$ -th and  $t_3$ -th dimensions of  $\mathbf{r}_i$  to 1 while setting the other dimensions to 0.  
410 The quality is calculated by  $q_i = (\mathbf{Q}^T \mathbf{r}_i + U)/2$ , where  $U$  is generated uniformly from  $[0, 1]$ . To  
411 simulate the real environment, only  $\mathbf{r}_i$  of each document can be observed.

412 At each time, the hidden state consists of

- 413 • user id  $i$ , indicating the current user;
- 414 • interest  $I$ , determining the satisfaction of the user;
- 415 • satisfaction  $s$ , influencing the reward of policy;
- 416 • document vector  $\mathbf{d}$ , the relevance vector of the current document.

417 We generated 5 preference vectors  $\mathbf{p}_i \in [-1, 1]^T$ . Each of them represents one user. When the user  
418 sampler generates the initial state, it randomly pick one from the 5 users, generate an initial interest  
419  $I$ , and set the satisfaction by  $s = \frac{1}{1+e^{-0.5I}}$ . The initial document vector is set as  $[1, 1, \dots, 1]^T$ . To  
420 simulate the real environment, only  $i$  and  $\mathbf{d}$  can be observed by the agent.

421 Now we define the reward function and the state transition function. Suppose we recommend  
422 the  $j$ -th document to the  $i$ -th user. We define the liking of the user to the document by  $l_{i,j} =$   
423  $\vec{e}^T(\mathbf{r}_j \circ \mathbf{p}_i \circ (\mathbf{d} + 0.5)/2)$ , where  $\circ$  is element-wise multiplication. This formula indicates the  
424 expectation of the user about the next document. It should be close to his or her preference as well as  
425 the current document. The probability of taking the document is  $\frac{l_{i,j}}{1+l_{i,j}}$  while the probability of leaving  
426 is  $\frac{1}{1+l_{i,j}}$ . If the user takes the document, we will calculate its engagement time by  $t_{i,j} \sim \mathcal{N}(q_j, 0.1^2)$   
427 and produce the reward of  $s * e^{t_{i,j}}$ . The reward depends on the quality of the document as well as the  
428 user satisfaction.

429 After the choice of user, the state vector will change. The interest will be updated by  $I' = 0.9I +$   
430  $\mathbf{p}_i^T \mathbf{r}_j + V$ , where  $V \sim \mathcal{N}(0, 0.1^2)$ . Meanwhile, the document vector is updated by  $\mathbf{d}'_i = \mathbf{r}_j$ . Note  
431 we also need to update the interest by  $s' = \frac{1}{1+e^{-0.5I'}}$ .

### 432 D.2 Implementation of REINFORCE

433 In the above environment, at each step, the agent needs to propose a document only with  $i, \mathbf{d}$  and  
434 document list  $[\mathbf{r}_1, \mathbf{r}_2, \dots, \mathbf{r}_D]$ . We can train a policy network to represent the policy  $\pi(a|s)$ . However,  
435 when the list is long(action space is large), it is hard to directly output the policy  $\pi(a|s)$  from neural  
436 networks. To exploit the structure of documents, we reduce the output of the policy network to a  
437  $T$  dimension vector  $\mathbf{y}$  and compute the policy by  $\pi(a_i|s) \propto \mathbf{y}^T \mathbf{r}_i$ . This not only solves the above  
438 problem but also reduces the time complexity of sampling. We initialize  $\mathbf{b}_i = \sum_{j=1}^i \mathbf{r}_j$ . When  
439 sampling, we can generate a number  $c$  from  $[0, 1]$  and use binary search to find the smallest  $k$   
440 satisfying  $\mathbf{y}^T \mathbf{b}_k \geq c$ . The  $k$ -th document would then be the sampled document. The time complexity  
441 is  $O(T \log D)$ , which is useful when the document list is long.

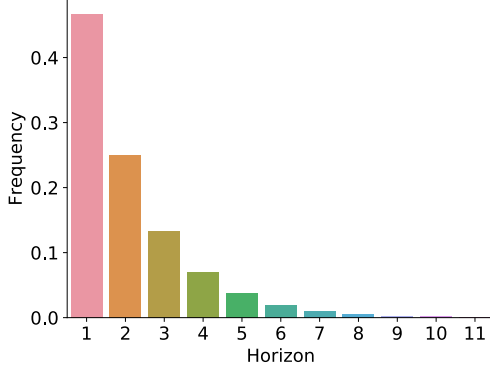

Figure 2: Distribution of length of data.

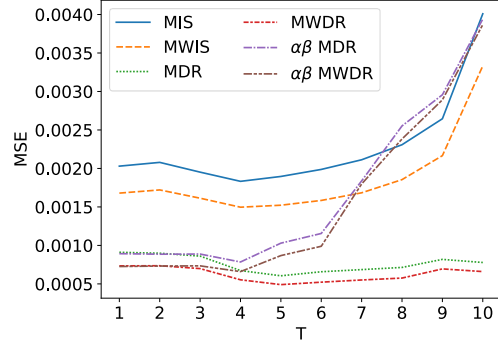

Figure 3: MSE of the methods with different T.

### D.3 Implementation of OPE Algorithms

In the same environment, we train 100 different REINFORCE policies  $p_1, p_2, \dots, p_{100}$ . Each policy collects 1000000 offline data, with the  $i$ -th defined by  $DATA_i$ . In our experiments, the policies are set up as target policy and behavior policies in turn. Specifically, for the  $i$ -th experiment, we set the target policy as  $p_i$  and use  $DATA_i$  to estimate the true mean reward  $\bar{\theta}_i$ . The behavior policies are set as  $\forall j \in \{1, 2, \dots, M\} \pi_j = p_{(i+j-1)\%100+1}$  and the offline data are  $(DATA_{i+1}, DATA_{i+2}, \dots, DATA_{(i+j-1)\%100+1})$ . With the settings, the  $i$ -th evaluation result is  $\hat{\theta}_i$  and the squared error is computed by  $(\hat{\theta}_i - \bar{\theta}_i)^2$ . We use the first 50 experiments as validation set to tune parameters and the last 50 experiments as test set to report the results.

We trained DM with 10000 data. The reward function  $\mathbb{E}[R(s, a)]$  is approximated by Bayesian Ridge Regressor [19]. The transition function  $P(\cdot|s, a)$  is approximated by neural network. The network consists of 2 fully connected layers with 512 units and an output layer with 2 units. The hidden layers are activated by relu and the last layer is activated by softmax. We minimize the cross entropy loss function with Adam optimizer [12]. The batch size is 32 and we train for 600 epochs. For the first 300 epochs the learning rate is set as 0.0001. For the last 300 epochs the learning rate is 0.00001. After approximating the environment functions, we iterate by formula (1) for 20 times and get the estimated value functions  $\hat{Q}(s, a)$  and  $\hat{V}(s)$ .

To reduce the variance of the methods we clip the importance ratios. For IS based methods we replace  $\rho_{i,j,t}$  by  $\bar{\rho}_{i,j,t} = \min(\rho_{i,j,t}, 2000)$ . For DR based methods we make  $\hat{V}_{i,j,t} = \gamma^t (\bar{\rho}_{i,j,t-1} \frac{\pi(a_{i,j,t}|s_{i,j,t})}{\pi_i(a_{i,j,t}|s_{i,j,t})} (r_{i,j,t} - \hat{Q}(s_{i,j,t}, a_{i,j,t})) + \bar{\rho}_{i,j,t-1} \hat{V}(s_{i,j,t}))$ . Note that clipping introduces additional bias. So our methods can be further improved by considering the bias.

### D.4 Tuning of Hyperparameter T

In mixture estimators and  $\alpha\beta$  mixture estimators, we choose a hyper-parameter  $T$ , mix the values from 0 to  $T$  and simply add up the remains. This is because the length of data from each behavior policy is random, as Figure 2. When  $t$  is large, the reward decreases exponentially and the variances and covariances about  $\hat{V}_{i,t}$  also decreases, making the matrixes nearly singular. Such problem leads to the phenomenon in Figure 3. Numerical results can be found in Appendix E.1. When  $T$  is small, the MSE decreases as  $T$  increases because more values are mixed. When  $T$  is large, the MSE increases as  $T$  increases because of the amplification of error from ill covariance matrixes. By Figure 3, we set  $T=4$  for MIS, MWIS,  $\alpha\beta$  MDR and  $\alpha\beta$  MWDR and set  $T=5$  for MDR and MWDR.

## 472 E Numerical Results

### 473 E.1 MSE of different methods with different T

|     | T  | MIS             | MWIS            | MDR             | MWDR            | $\alpha\beta$ MDR | $\alpha\beta$ MWDR |
|-----|----|-----------------|-----------------|-----------------|-----------------|-------------------|--------------------|
|     | 1  | 0.00203         | 0.001679        | 0.00091         | 0.000734        | 0.000893          | 0.000726           |
|     | 2  | 0.002079        | 0.001721        | 0.000898        | 0.000736        | 0.000886          | 0.000732           |
|     | 3  | 0.001952        | 0.001613        | 0.000861        | 0.000699        | 0.000888          | 0.000735           |
|     | 4  | <b>0.001833</b> | <b>0.001497</b> | 0.000673        | 0.000553        | <b>0.000785</b>   | <b>0.00066</b>     |
| 474 | 5  | 0.001896        | 0.001522        | <b>0.000605</b> | <b>0.000491</b> | 0.001029          | 0.000868           |
|     | 6  | 0.001987        | 0.001584        | 0.000658        | 0.000522        | 0.001155          | 0.000989           |
|     | 7  | 0.002113        | 0.001684        | 0.000686        | 0.000551        | 0.001838          | 0.001798           |
|     | 8  | 0.002308        | 0.001855        | 0.000714        | 0.000576        | 0.002552          | 0.002383           |
|     | 9  | 0.002646        | 0.002166        | 0.000818        | 0.000695        | 0.002957          | 0.002891           |
|     | 10 | 0.004009        | 0.003332        | 0.000778        | 0.00066         | 0.003941          | 0.003869           |

### 475 E.2 MSE of different methods with different M

|     | M                  | 1               | 2               | 3               | 4              | 5               |
|-----|--------------------|-----------------|-----------------|-----------------|----------------|-----------------|
|     | IS                 | 0.001877        | 0.001703        | 0.001544        | 0.001515       | 0.001344        |
|     | WIS                | 0.001525        | 0.001351        | 0.00123         | 0.001217       | 0.001075        |
|     | SWIS               | 0.001525        | 0.001367        | 0.001252        | 0.001241       | 0.001099        |
|     | NMIS               | 0.001942        | 0.001435        | 0.001289        | 0.001158       | 0.001017        |
|     | NMWIS              | 0.001576        | 0.001139        | 0.001041        | 0.000953       | 0.000836        |
|     | MIS                | 0.001907        | 0.001452        | 0.001394        | 0.0013         | 0.001126        |
|     | MWIS               | 0.001533        | 0.001152        | 0.001126        | 0.001075       | 0.000928        |
| 476 | DR                 | 0.00082         | 0.000455        | 0.000309        | 0.000381       | 0.000377        |
|     | WDR                | <b>0.000675</b> | 0.000357        | <b>0.000235</b> | 0.0003         | 0.000301        |
|     | SWDR               | <b>0.000675</b> | 0.000352        | <b>0.000235</b> | 0.0003         | 0.000299        |
|     | NMDR               | 0.000968        | 0.000422        | 0.000284        | 0.0004         | 0.000395        |
|     | NMWDR              | 0.000883        | 0.000375        | 0.000253        | 0.000337       | 0.000333        |
|     | MDR                | 0.000861        | 0.000398        | 0.000294        | 0.000264       | 0.000311        |
|     | MWDR               | 0.000776        | <b>0.000334</b> | 0.000247        | <b>0.00021</b> | <b>0.000245</b> |
|     | $\alpha\beta$ MDR  | 0.001017        | 0.000469        | 0.00041         | 0.000408       | 0.000371        |
|     | $\alpha\beta$ MWDR | 0.000911        | 0.000394        | 0.000349        | 0.000344       | 0.000317        |

### 477 E.3 MSE and condition number of different methods

|     | Method             | MSE                          | Cond Number        |
|-----|--------------------|------------------------------|--------------------|
|     | IS                 | 0.0013444257969445908        | /                  |
|     | WIS                | 0.0010745378682455794        | /                  |
|     | SWIS               | 0.001099086646547933         | /                  |
|     | NMIS               | 0.0010165986763763788        | /                  |
|     | NMWIS              | 0.0008363384188827019        | /                  |
|     | MIS                | 0.0011259428162672161        | 15.233859883668414 |
|     | MWIS               | 0.0009282956141402447        | 17.60016020307187  |
| 478 | DR                 | 0.00037712737924285305       | /                  |
|     | WDR                | 0.0003011794977270172        | /                  |
|     | SWDR               | 0.00029893021636011546       | /                  |
|     | NMDR               | 0.0003947548680215243        | /                  |
|     | NMWDR              | 0.00033273193073131153       | /                  |
|     | MDR                | 0.0003109721026979073        | 51.790423695019456 |
|     | MWDR               | <b>0.0002449612080194226</b> | 74.18300868487523  |
|     | $\alpha\beta$ MDR  | 0.00037141793259772417       | 320.712344891526   |
|     | $\alpha\beta$ MWDR | 0.0003171837312053011        | 337.9175903029748  |
